# Supplementary material for: SuperQuadricOcc: Real-Time Self-Supervised Semantic Occupancy Estimation with Superquadric Volume Rendering
Source: arXiv:2511.17361 source file (2026-08-11)
Supplement: Supplementary file 1 [file benchmark.tex]

\begin{table}[htpb]
\caption{\textbf{Render Benchmark:} Render time for 10,000 SuperQuadrics, $512\times1408$ resolution, and max scene resolution. Max scene resolution refers to voxel resolution of $400\times400\times32$ for voxel-based methods, and/or ray samples $L=200$ for volume render methods. The best result overall is highlighted in \textbf{bold}.} 
\centering 
\begin{adjustbox}{width=0.40\linewidth}
\begin{tabular}{l|cc}
    \toprule
    \textbf{Model} & \textbf{Latency} & \textbf{Memory} \\
    \midrule
    MLGA & - \\
    Gaussianization & - \\
    Voxel NeRF & - \\
    SQOcc-R & - \\
    \bottomrule
\end{tabular}
\end{adjustbox}
\label{tab:benchmark}
\end{table}
