# Supplementary material for: SuperQuadricOcc: Real-Time Self-Supervised Semantic Occupancy Estimation with Superquadric Volume Rendering
Source: arXiv:2511.17361 source file (2026-08-11)
Supplement: Supplementary file 2 [file ablation_main.tex]

\begin{table*}[h]
\centering
\scriptsize
\setlength{\tabcolsep}{2.0pt}
\renewcommand{\arraystretch}{1.05}
\caption{\textbf{SuperQuadricOcc-Render ablation studies} on Occ3D-nuScenes \cite{tian2023occ3d} and OpenOccv2 \cite{tong2023scene} datasets. The grey row is the preferred setting. Lat. denotes rendering latency in milliseconds.}

\begin{adjustbox}{max width=\textwidth}
\begin{tabular}{@{}c@{\hspace{0.35em}}c@{\hspace{0.35em}}c@{\hspace{0.35em}}c@{}}

\begin{tabular}{c|cc|cc|c}
\toprule
\multirow{2}{*}{$\mathcal{N}$}
& \multirow{2}{*}{\textbf{IoU}}
& \multirow{2}{*}{\textbf{mIoU}}
& \multicolumn{2}{c|}{\textbf{RayIoU}}
& \multirow{2}{*}{\textbf{Lat.}} \\
&
&
& \textbf{Occ3D} & \textbf{OpenOccv2}
& \\
\midrule
3 & 38.86 & 14.53 & 14.19 & 15.23 & \textbf{13.54} \\
\rowcolor{black!5}
5 & \textbf{41.10} & 15.80 & 17.21 & 17.87 & 17.18 \\
\rowcolor{white}
7 & 40.65 & \textbf{15.88} & \textbf{18.06} & \textbf{18.43} & 29.73 \\
\bottomrule
\end{tabular}

&

\begin{tabular}{c|cc|cc|c}
\toprule
\multirow{2}{*}{$\kappa$}
& \multirow{2}{*}{\textbf{IoU}}
& \multirow{2}{*}{\textbf{mIoU}}
& \multicolumn{2}{c|}{\textbf{RayIoU}}
& \multirow{2}{*}{\textbf{Lat.}} \\
&
&
& \textbf{Occ3D} & \textbf{OpenOccv2}
& \\
\midrule
$1e^{-2}$ & 39.45 & 15.24 & 16.68 & 17.42 & \textbf{15.36} \\
$1e^{-4}$ & \textbf{41.15} & 15.69 & \textbf{17.44} & \textbf{18.05} & 16.86 \\
\rowcolor{black!5}
None & 41.10 & \textbf{15.80} & 17.21 & 17.87 & 17.18 \\
\bottomrule
\end{tabular}

&

\begin{tabular}{c|cc|cc|c}
\toprule
\multirow{2}{*}{$N$}
& \multirow{2}{*}{\textbf{IoU}}
& \multirow{2}{*}{\textbf{mIoU}}
& \multicolumn{2}{c|}{\textbf{RayIoU}}
& \multirow{2}{*}{\textbf{Lat.}} \\
&
&
& \textbf{Occ3D} & \textbf{OpenOccv2}
& \\
\midrule
1,200  & 39.69 & 14.96 & 16.28 & 16.99 & \textbf{16.33} \\
\rowcolor{black!5}
1,600  & 41.10 & 15.80 & 17.21 & 17.87 & 17.18 \\
\rowcolor{white}
2,000  & 41.36 & \textbf{16.08} & \textbf{17.71} & \textbf{18.25} & 20.16 \\
4,000  & 40.24 & 15.92 & 17.51 & 17.99 & 34.84 \\
10,000 & \textbf{42.00} & 15.86 & 16.38 & 17.03 & 91.18 \\
\bottomrule
\end{tabular}

&

\begin{tabular}{c|cc|cc|c}
\toprule
\multirow{2}{*}{$L$}
& \multirow{2}{*}{\textbf{IoU}}
& \multirow{2}{*}{\textbf{mIoU}}
& \multicolumn{2}{c|}{\textbf{RayIoU}}
& \multirow{2}{*}{\textbf{Lat.}} \\
&
&
& \textbf{Occ3D} & \textbf{OpenOccv2}
& \\
\midrule
50  & 40.61 & 15.64 & 17.30 & 17.85 & \textbf{12.68} \\
75  & 40.89 & 15.49 & 16.90 & 17.65 & 15.30 \\
\rowcolor{black!5}
100 & 41.10 & 15.80 & 17.21 & 17.87 & 17.18 \\
\rowcolor{white}
125 & 41.14 & 15.83 & 17.14 & 17.87 & 19.77 \\
150 & \textbf{41.53} & \textbf{15.85} & \textbf{17.52} & \textbf{18.06} & 21.12 \\
\bottomrule
\end{tabular}

\end{tabular}
\end{adjustbox}

\label{tab:main_abl}
\end{table*}
