# Supplementary material for: SuperQuadricOcc: Real-Time Self-Supervised Semantic Occupancy Estimation with Superquadric Volume Rendering
Source: arXiv:2511.17361 source file (2026-08-11)
Supplement: Supplementary file 3 [file depth_80m.tex]

\begin{table}[htpb]
\caption{\textbf{Depth Estimation performance on nuScenes} For 80m range.}
\centering
\begin{adjustbox}{width=\linewidth}
\begin{tabular}{l|cc|cc|ccc}
    \toprule
    & \textbf{Abs}
    & \textbf{Sq}
    & \multicolumn{2}{c|}{\textbf{RMSE} }
    %& \textbf{RMSE}
    & \multicolumn{3}{c}{$\boldsymbol{\delta}$}
    % & $\boldsymbol{\delta\!<\!1.25} \uparrow$
    % & $\boldsymbol{\delta\!<\!1.25^2} \uparrow$
    % & $\boldsymbol{\delta\!<\!1.25^3} \uparrow$
    \\
    \multirow{-2}{*}{\textbf{Method}}
    & \textbf{Rel} $\downarrow$
    & \textbf{Rel} $\downarrow$
    & $\downarrow$
    & \textbf{log} $\downarrow$
    & $\boldsymbol{<\!\!1.25} \uparrow$
    & $\boldsymbol{<\!\!1.25^2} \uparrow$
    & $\boldsymbol{<\!\!1.25^3} \uparrow$ \\
    \midrule
    MLGA &
    0.194 & 1.934 & 8.236 & 0.569 & 0.714 & 0.854 & 0.914 \\
    Gaussianisation &
    0.203 & 1.880 & \textbf{8.071} & \textbf{0.351} & 0.711 & 0.852 & 0.919 \\
    Voxel NeRF & 
    0.208 & 2.023 & 8.383 & 0.387 & 0.683 & 0.822 & 0.894 \\
    \renderShort{} (Ours) &
    \textbf{0.190} & \textbf{1.825} & 8.163 & 0.353 & \textbf{0.717} & \textbf{0.857} & \textbf{0.920} \\
\bottomrule
\end{tabular}
\end{adjustbox}
\label{tab:80m_depth}
\end{table}
