# Supplementary material for: SuperQuadricOcc: Real-Time Self-Supervised Semantic Occupancy Estimation with Superquadric Volume Rendering
Source: arXiv:2511.17361 source file (2026-08-11)
Supplement: Supplementary file 4 [file rayIoU_class.tex]

\begin{table*}[htp]
    \caption{\textbf{SuperQuadricOcc render method RayIoU comparison per class on Occ3D-nuScenes \cite{tian2023occ3d}:} All models are self-supervised. Classwise metrics are taken from RayIoU@2. The best-performer is highlighted in \textbf{bold}.}
     %\andreic{Are mem. and fps identical for SuperQuadricOcc and SQ-Nerf identical?}
  \centering
  \setlength{\tabcolsep}{3pt}
  \begin{adjustbox}{width=\textwidth}
  \begin{tabular}{
    @{}l
    | >{\columncolor{blue!5}}c
    |  >{\columncolor{blue!5}}c
        >{\columncolor{blue!5}}c
        >{\columncolor{blue!5}}c
    |*{15}{c}
    @{}
}
    \toprule
\textbf{Model} 
& \rotatebox{\myangle}{\textbf{RayIoU}}
& \rotatebox{\myangle}{\textbf{RayIoU@1}}
& \rotatebox{\myangle}{\textbf{RayIoU@2}}
& \rotatebox{\myangle}{\textbf{RayIoU@4}}
& \rotatebox{\myangle}{\textcolor{barrier}{$\blacksquare$} barrier} & \rotatebox{\myangle}{\textcolor{bicycle}{$\blacksquare$} bicycle} & \rotatebox{\myangle}{\textcolor{bus}{$\blacksquare$} bus} & \rotatebox{\myangle}{\textcolor{car}{$\blacksquare$} car} & \rotatebox{\myangle}{\textcolor{construction}{$\blacksquare$} const. veh.} & \rotatebox{\myangle}{\textcolor{motorcycle}{$\blacksquare$} motorcycle} & \rotatebox{\myangle}{\textcolor{pedestrian}{$\blacksquare$} pedestrian} & \rotatebox{\myangle}{\textcolor{cone}{$\blacksquare$} traffic cone} & \rotatebox{\myangle}{\textcolor{trailer}{$\blacksquare$} trailer} & \rotatebox{\myangle}{\textcolor{truck}{$\blacksquare$} truck} & \rotatebox{\myangle}{\textcolor{driveable}{$\blacksquare$} drive. surf.} & \rotatebox{\myangle}{\textcolor{sidewalk}{$\blacksquare$} sidewalk} & \rotatebox{\myangle}{\textcolor{terrain}{$\blacksquare$} terrain} & \rotatebox{\myangle}{\textcolor{manmade}{$\blacksquare$} manmade} & \rotatebox{\myangle}{\textcolor{vegetation}{$\blacksquare$} vegetation} \\
    \midrule 
   MLGA & 12.1 & 7.3 & 11.9 & 17.2 & 8.4 & 6.0 & 31.2 & 23.6 & 3.9 & 5.5 & 9.6 & 4.8 & \textbf{1.2} & 24.3 & 20.2 & 5.0 & 6.0 & 16.4 & 15.9
    \\
    Gaussianisation & 16.4 & 10.6 & 16.2 & 22.3 & 12.0 & 7.1 & 25.9 & 20.2 & \textbf{5.0} & 6.7 & 15.1 & 12.8 & 0.2 & 24.4 & 42.8 & 12.9 & 14.5 & 22.6 & 23.5
    \\
    Voxel NeRF & 18.8 & 13.0 & 18.8 & 24.5 & \textbf{16.3} & 7.0 & 35.1 & 29.5 & 2.7 & 7.2 & 17.2 & \textbf{16.1} & 0.0 & 28.5 & \textbf{47.0} & \textbf{15.2} & \textbf{15.2} & 23.3 & 21.4
    \\
    SQOcc-R (Ours) & \textbf{19.6} & \textbf{13.5} & \textbf{19.6} & \textbf{25.6} & 14.3 & \textbf{8.8} & \textbf{38.0} & \textbf{31.2} & 4.9 & \textbf{8.6} & \textbf{18.1} & 15.1 & 0.3 & \textbf{30.7} & 45.9 & 14.3 & \textbf{15.2} & \textbf{24.1} & \textbf{23.9}
    \\
    %GaussianFlowOcc & - & - & - & - & 12.60 & 7.20 & 39.80 & 30.70 & 5.50 & 11.20 & 16.50 & 13.70 & 0.10 & 28.70 & 35.40 & 13.30 & 14.40 & 23.70 & 22.30 \\
    \bottomrule
  \end{tabular}
  \end{adjustbox}
  \label{tab:rayiou_class}
\end{table*}



% \begin{table*}[t]
%     \caption{\textbf{State-of-the-art model comparison on Occ3D-nuScenes \cite{tian2023occ3d}:} Rep. denotes the method of scene representation: Gauss - Gaussian; Quad - SuperQuadric. Mem. denotes the maximum memory (GB) during inference (rendering pipeline not included). All models are self-supervised. The best-performer is highlighted in \textbf{bold}.}
%      %\andreic{Are mem. and fps identical for SuperQuadricOcc and SQ-Nerf identical?}
%   \centering
%   \setlength{\tabcolsep}{3pt}
%   \begin{adjustbox}{width=\textwidth}
%   \begin{tabular}{
%     @{}l
%     |>{\columncolor{red!5}}c
%     |>{\columncolor{green!5}}c
%         >{\columncolor{green!5}}c
%     | >{\columncolor{blue!5}}c
%         >{\columncolor{blue!5}}c
%     |*{15}{c}
%     @{}
% }
%     \toprule
% \textbf{Model} & \textbf{Rep.} & \textbf{Mem.} & \textbf{FPS} & \textbf{IoU} & \textbf{mIoU} & \rotatebox{\myangle}{\textcolor{barrier}{$\blacksquare$} barrier} & \rotatebox{\myangle}{\textcolor{bicycle}{$\blacksquare$} bicycle} & \rotatebox{\myangle}{\textcolor{bus}{$\blacksquare$} bus} & \rotatebox{\myangle}{\textcolor{car}{$\blacksquare$} car} & \rotatebox{\myangle}{\textcolor{construction}{$\blacksquare$} const. veh.} & \rotatebox{\myangle}{\textcolor{motorcycle}{$\blacksquare$} motorcycle} & \rotatebox{\myangle}{\textcolor{pedestrian}{$\blacksquare$} pedestrian} & \rotatebox{\myangle}{\textcolor{cone}{$\blacksquare$} traffic cone} & \rotatebox{\myangle}{\textcolor{trailer}{$\blacksquare$} trailer} & \rotatebox{\myangle}{\textcolor{truck}{$\blacksquare$} truck} & \rotatebox{\myangle}{\textcolor{driveable}{$\blacksquare$} drive. surf.} & \rotatebox{\myangle}{\textcolor{sidewalk}{$\blacksquare$} sidewalk} & \rotatebox{\myangle}{\textcolor{terrain}{$\blacksquare$} terrain} & \rotatebox{\myangle}{\textcolor{manmade}{$\blacksquare$} manmade} & \rotatebox{\myangle}{\textcolor{vegetation}{$\blacksquare$} vegetation} \\
%     \midrule 
%     DistillNeRF \cite{wang2024distillnerf} & Voxel & - & 2.8 & 29.1 & 10.1 & 1.4 & 2.1 & 10.2 & 10.1 & 2.6 & 2.0 & 5.5 & 4.6 & 1.4 & 7.9 & 43.0 & 16.9 & 15.0 & 14.1 & 15.1 \\
%     SelfOcc \cite{huang2024selfocc} & Voxel & 3.00 & 7.4 & 45.0 & 10.5 & 0.2 & 0.7 & 5.5 & 12.5 & 0.0 & 0.8 & 2.1 & 0.0 & 0.0 & 8.3 & 55.5 & 26.3 & 26.5 & 14.2 & 5.6 \\
%     OccNeRF \cite{zhang2023occnerf} & Voxel & 12.68 & 5.4 & \textbf{46.4} & 10.8 & 0.8 & 0.8 & 5.1 & 12.5 & 3.5 & 0.2 & 3.1 & 1.8 & 0.5 & 3.9 & 52.6 & 20.8 & 24.8 & 18.5 & 13.2 \\
%     GaussianOcc \cite{gaussianocc} & Voxel & 11.81 & 5.4 & 42.9 & 11.3 & 1.8 & 5.8 & 14.6 & 13.6 & 1.3 & 2.8 & 8.0 & 9.8 & 0.6 & 9.6 & 44.6 & 20.1 & 17.6 & 8.6 & 10.3 \\
%     %SuperQuadricOcc \cite{hayes2025superquadricocc} & Quad & \textbf{0.70} & \textbf{21.5} & 33.67 & 12.69 & 5.78 & 5.69 & 16.32 & 13.06 & 3.72 & 5.69 & 3.94 & 3.54 & 2.56 & 11.94 & 43.58 & 20.66 & 24.15 & 14.45 & 15.29 \\
%     GaussTR \cite{jiang2025gausstr} & Gauss & 1.97 & 0.3 & 44.5 & 13.8 & 6.5 & 8.5 & \textbf{21.8} & \textbf{24.3} & 6.3 & \textbf{15.5} & 7.9 & 1.9 & \textbf{6.1} & \textbf{17.2} & 37.0 & 17.2 & 7.2 & \textbf{21.2} & 10.0 \\
%     EasyOcc \cite{hayes2025easyocc} & Voxel & - & 5.4 & 38.9 & 15.7 & 1.9 & 6.7 & \textbf{15.1} & 21.7 & 2.7 & 8.1 & 15.3 & 11.1 & 1.4 & 12.8 & 55.8 & 27.9 & 22.1 & 16.1 & 17.3 \\
%     %\midrule
%     GaussianFlowOcc \cite{boeder2025gaussianflowocc} & Gauss & 2.85 & 9.6 & 40.5 & 16.7 & 6.7 & 9.2 & 17.5 & 16.5 & 4.0 & 11.9 & 8.8 & 9.7 & 0.6 & 12.3 & 49.3 & 30.8 & \textbf{34.6} & 17.4 & 20.8 
%     \\
%     TT-Occ \cite{zhang2025tt} & Gauss & 9.90 & 0.7 & - & 16.7 & \textbf{21.5} & \textbf{10.5} & 10.7 & 14.7 & \textbf{11.9} & 12.3 & 9.7 & \textbf{12.2} & 4.4 & 7.9 & 48.3 & 23.7 & 28.3 & 14.1 & 20.2 \\
%     \midrule
%     SuperQuadricOcc (Ours) & Quad & \textbf{0.70} & \textbf{21.5} & 43.5 & \textbf{17.1} & 7.0 & 8.3 & 16.6 & 14.8 & 3.4 & 9.1 & 8.0 & 8.8 & 1.1 & 12.0 & \textbf{64.7} & \textbf{31.4} & 34.3 & 16.6 & \textbf{21.0}
%     \\
%     \bottomrule
%   \end{tabular}
%   \end{adjustbox}
%   \label{tab:sota_occ3d}
% \end{table*}
